# Supplementary material for: Game Theoretic Optimization via Gradient-based Nikaido-Isoda Function
Source: arXiv:1905.05927 source file (2019-05-15)
Supplement: Supplementary file 1 [file appendix.tex]

\section{Gradient and Hessian of $V_i(\bfx;\eta)$}

\begin{lemma}\label{lemma:gradV}
\begin{equation}
\begin{aligned}
	& 	\nabla V_i(\bfx;\eta) \\
	=		&	\nabla f_i(\bfx) - (I - \eta \nabla^2 f_i(\bfx) E_i ) \nabla f_i(\bfy(\bfx;i,\eta)) \label{defgradVa}
		\end{aligned}
\end{equation}
where $E_i = F_i F_i^T$ with $F_i \in \R^{n \times n_i}$ defined as 
$F_i^T = \begin{bmatrix} \bfzero_{n_i \times \sum_{j=1}^{i-1}n_j }  & 
I_{i} & \bfzero_{n_i \times \sum_{j=i+1}^N n_j} \end{bmatrix}$
and $I \in \R^{n \times n}$ and $I_{i} \in \R^{n_i \times n_i}$ are identity matrices.
\end{lemma}
\begin{proof}
\begin{subequations}
 Based on the definition of $\bfy(\bfx;i,\eta)$ in~\eqref{defVy}, the derivative of 
$\bfy(\bfx;i,\eta)$ w.r.t $\bfx$ is
\begin{equation}
	\begin{aligned}
				&	\nabla_i y_i(\bfx;i,\eta) = I_i - \eta\nabla^2_{ii}f_i(\bfx), 
					\nabla_j y_i(\bfx;\eta) = - \eta\nabla^2_{ij} f_i(\bfx)   
	\end{aligned}\label{defgrady1}
\end{equation}
Using the chain rule for differentiation,
\begin{equation}
	\begin{aligned}
		\nabla_i V_i(\bfx;\eta) =															&		\nabla_i f_i(\bfx) -\nabla_i \bfy(x;i,\eta) \nabla_i f_i(\bfx) \\ 
\overset{\eqref{defgrady1}}{=}				&		\nabla_i f_i(\bfx) 
				- \nabla_i f_i(\bfy(\bfx;i,\eta)) \\
		& 		+ \eta\nabla^2_{ii} f_i(\bfx) \nabla_i f_i(\bfy(\bfx;i,\eta)) \\
		\nabla_j V_i(\bfx;\eta) 	
 \overset{\eqref{defgrady1}}{=}			&		\nabla_j f_i(\bfx) - 
 				\nabla_j f_i(\bfy(\bfx;i,\eta)) \\ 
		&		+ \nabla_i \bfy(\bfx;i,\eta) \nabla_i f_i(\bfx) \\ 
\overset{\eqref{defgrady1}}{=}				&		\nabla_j f_i(\bfx) - 
				\nabla_j f_i(y_i(\bfx;i,\eta)) \\ 
		&		+ \eta\nabla^2_{ji} f_i(\bfx) \nabla_i f_i(\bfx).
	\end{aligned}\label{defgradV112}
\end{equation}
The expression for $\nabla V_1$ in~\eqref{defgradV} can be obtained by combining the 
expressions in~\eqref{defgradV112}.  The expression for $\nabla V_2$ can be derived in an identical manner.
\end{subequations}
\end{proof}

\begin{lemma}\label{lemma:hessianV}
\begin{equation}
	\begin{aligned}
		& \nabla^2 V_i(\bfx;\eta) 
	=		\nabla^2 f_i(\bfx) 
		+ \eta \nabla^3 f_i(\bfx) [E_i \nabla f_i(\bfy_i(\bfx;i,\eta)] \\
		& - (I - \eta \nabla^2 f_i(x) E_i ) \nabla^2  f_i(\bfy(\bfx;i,\eta)) (I - \eta E_i \nabla^2 f_i(\bfx)) 
		\end{aligned}
\end{equation}
where $\nabla^3 f_i(\bfx) [d] = \lim_{\alpha \rightarrow 0} \frac{\nabla^2 f_i(\bfx+\alpha d) - 
\nabla^2 f_i(\bfx)}{\alpha}$ is the action of the third derivative along the direction $d$. 	
\end{lemma}
\begin{proof}
The proof follows from the chain rule of differentiation and can be obtained along the 
lines of the proof to Lemma~\ref{lemma:gradV}.
\end{proof}

\section{Residual Minimization}\label{sec:residual_min}
\input{residual.tex}
